# Supplementary material for: MomentaMorph: Unsupervised Spatial-Temporal Registration with Momenta, Shooting, and Correction
Source: arXiv:2308.02949 source file (2023-08-05)
Supplement: Supplementary file 1 [file appendix.tex]

- Future: Deep feature, NODEO,
 Test CPSAMM,
 "Go with only SPAMM?"
 reduce scanning time for 3D acquisition
 do grid tags (full k-sapce)in sagital plane instead of line tags (slab of k-sapce). why? radial/spiral acq. fast. 
 go back to cardiac imaging

 -NCC: Normalized cross-correlation (NCC) is known to be more robust to local intensity variations and has been found to be superior in brain MR registration applications (Avants et al., 2008).
 
 -SSIM: The structural similarity index (SSIM) (Wang et al., 2004) has also been demonstrated to be an effective loss function for mono-modal image registration (Chen et al., 2020; Mahapatra et al., 2018a; Sandkühler et al., 2018). SSIM takes into account luminance, contrast, and structure. The weighting of three terms might matter. SSIM's strcuture term is robust to contrast change and illuminance change. (Code: AirLab)
 
 - Mutual information: For multi-modal applications, traditional methods often use mutual information (MI). (Viola and Wells III, 1997). valuate the relationship between the two images by calculating intensity statistics, such as intensity histograms, to measure statistical dependence. (ANTS)
 
 -dMI: the standard method for calculating intensity histograms, which involves counting, is not differentiable, so a Parzen window formulation (Thévenaz anUnser, 2000) is often used to allow the loss to be backpropagated during network training. 
 these intensity-statistic-based measurements do not take into account local structural information, making them more suitable for rigid/affine registration and less suitable for deformable registration applications (Pluim et al., 2000; Heinrich et al., 2013). (MONAI)
 
 -NGF compares images by focusing on the intensity changes, or edges, in the images. The similarity between the two images is determined by the presence of intensity changes at the same locations, regardless of the modalities of the images being compared. NGF was originally developed for multi-modal applications like brain MR T1-to-T2 and PET-to-CT (Haber and Modersitzki, 2006). However, it is now mostly used in learning-based registration models for lung CT registration (Hering et al., 2019, 2021; Mok and Chung, 2021a). (Code: AirLab)
 
 - SSC and MIND: modality-independent neighborhood descriptor (MIND) (Heinrich et al., 2012). (Code: https://github.com/multimodallearning/graphregnet/blob/master/utils.py)
 
 - DeepSIM (Code: https://github.com/SteffenCzolbe/DeepSimRegistration) Czolbe et al. (2021)
 
 -Haskins et al. (2019) 
 
 -Grzech et al. (2022)

  % Adjust the factor as needed
 \begin{tabular}{c|l|p{7cm}}
 	\toprule
 	\# & Equation & Comment \\
 	\hline
 	1 & \(M_z(x, 0^-) = M_0 \cdot \tagx\) & Right after tagging\\
 	2 & \(M_{xy}(x, 0^-) = 0\) & \\ \hline
 	3 & \(M_z(x, 0^+) = M_0 \cos \alpha\) & Right after tipping (in imaging process)\\
 	4 & \(M_{xy}(x, 0^+) = M_z(0^-) \cdot \sin \alpha = M_0 \cdot \sin \alpha\) & \\ \hline
 	5 & \(M_z(x, t) = M_z(x, 0^+) \cdot e^{-t / T_1} + M_0(1 - e^{-t / T_1})\) & when $ 0^+ \le t \le T_R$. Longitudinal relaxation \\
 	6 & \(\qquad = M_0 \cos \alpha \cdot e^{-t / T_1} + M_0(1 - e^{-t / T_1})\) & \\
 	7 & \(M_{xy}(x, t) = M_{xy}(x, 0^+) \cdot e^{-t / T_2^*}\) & Transverse relaxation by $T_2^*$ due to GRE. Multiuple lines in k-space are acquired. (To check) \\ \hline
 	\multicolumn{3}{c}{Assume: \(T_s^- \approx T_R^- \approx T_R^+\)}\\ \hline
 	8 & \(M_z(x, T_s^-) = M_0 \cos \alpha \cdot e^{-T_R / T_1} + M_0(1 - e^{-T_R / T_1})\) & The state right before the spoiler \\
 	9 & \(M_{xy}(x, T_s^-) = M_{xy}(x, 0^+) \cdot e^{-T_R / T_2^*}\) & \\ \hline
 	10 & \(M_z(x, T_R^-) = M_z(x, T_s^-)\) & Right after the spoiler. The spoiler does not affect z-magnetization \\
 	11 & \(M_{xy}(x, T_R^-) = 0\) & \\ \hline
 	12 & \(M_z(x, T_R^+) = M_z(x, T_R^-) \cdot \cos \alpha = M_z(x, T_s^-) \cdot \cos \alpha\) & Right after the second tip angle \\
 	13 & \(M_{xy}(x, T_R^+) = M_z(x, T_R^-) \cdot \sin \alpha\) & \\ \hline
 	14 & \(M_z(x, t) = M_z(x, T_R^+) \cdot e^{-\frac{t-T_R}{T_1}} + M_0(1 - e^{-\frac{t-T_R}{T_1}})\) & when $ T_R^+ \le t \le 2T_R$\\
 	15 & \(\qquad = M_z(x, T_s^-) \cdot \cos \alpha \cdot e^{-\frac{t-T_R}{T_1}} + M_0(1 - e^{-\frac{t-T_R}{T_1}})\) & Apply \# 12\\
 	16 & \( \qquad = M_0 \cdot \tagx \cdot \cos ^2 \alpha \cdot e^{-t / T_1}\) & Apply \# 8\\
 	& \( \qquad +M_0(1-e^{-T_R / T_1}) \cdot \cos  \alpha \cdot e^{-\frac{t-T_R}{T_1}}+M_0(1-e^{-\frac{t-T_R}{T_1}})\) & \\
 	17 & \(M_{xy}(x, t) = M_{xy}(x, T_R^+) \cdot e^{-\frac{t-T_R}{ T_2^*}}\) & \\
 	\bottomrule
 \end{tabular}
 
 In \#7, we acquire multiple scan multiple lines in the k-space, during this process, the magnitzuation undergone T2 start relaxation in the same time, which means the amplitude of those lines are different. 
 In \#16, we see only the first term varies on $x$, and thus tag maintains the sine-shape even during the transition to steady-state. 
 
 We then describe the simulation of tag-fading process. We ignore the fact that lines in k-space are acquired at different amplitude during $T_2^*$ decay. We known the amplitude of taglines are proportional to the $M_z(x,nT_R^-)$ and $M_{xy}(x,nT_R^+) = M_z(x,nT_R^-) \cdot \sin \alpha$. The $M_z(x,nT_R^-)$  can be expressed by $M_z(x,(n-1) T_R^-)$, thus the whole process can be computed iteratively with a initial condition:
 
 \begin{align}
 	M_z(x, n T_R^{-}) &= M_2\left(x,(n-1) T_R^{+}\right) \cdot e^{-\frac{T_R}{T_1}} + M_0\left(1-e^{-\frac{T_R}{T_1}}\right) \\
 	&= M_2\left(x,(n-1) T_R^{-}\right) \cos(\alpha) \cdot e^{-\frac{T_R}{T_1}} + M_0\left(1-e^{-\frac{T_R}{T_1}}\right) \\
 	M_z\left(x, 0^{-}\right) &= M_0 \tagx \\
 \end{align}
 
 Now we want to find the analytical solution for $M_z(x, n T_R^{-})$.  For simplicity, we denote :
 \begin{align}
 	&C_1 = \cos(\alpha) e^{-\frac{T_R}{T_1}} \\
 	&C_2 = M_0\left(1-e^{-\frac{T_R}{T}}\right) \\
 \end{align}
 
 Then we can write as 
 \begin{align}
 	&A_n = C_1 A_{n-1} + C_2 \quad (n \geqslant 1), \quad \text{where} \quad A_0 = M_0 \tagx \\
 	&A_n = C_1^n A_0 + C_2 \left(1 + C_1 + C_1^2 + \cdots + C_1^{n-1}\right) \\
 	&= C_1^n A_0 + C_2\left(\frac{1 - C_1^n}{1 - C_1}\right)
 \end{align}
 
 Substitude in, we got:
 \begin{equation}
 	\begin{aligned}
 		M_z(x, n T_R^-) & =\left(\cos \alpha \cdot e^{-\frac{T_R}{T_1}}\right)^n \cdot M_0 \cdot \tagx \\
 		& +M_0\left(1-e^{-\frac{T_R}{T_1}}\right) \cdot \frac{1-\left(\cos \alpha \cdot e^{-\frac{T_R}{T_1}}\right)^n}{1-\cos \alpha \cdot e^{-\frac{T_R}{T_1}}}
 	\end{aligned}
 \end{equation}
 
 \begin{table}[h]
 	\begin{tabular}{ccc}
 		\toprule
 		&&\\
 		\bottomrule
 	\end{tabular}%
 	\caption{Parameter settings for simulation.}
 \end{table}
